# Supplementary material for: Real identifiability vs complex identifiability
Source: arXiv:1608.07197 ancillary file (2016-10-20)
Supplement: Supplementary file 1 [file CRidentAnc.pdf]

**ANCILLARY FILE TO  
“REAL IDENTIFIABILITY VS COMPLEX IDENTIFIABILITY”**

ELENA ANGELINI, CRISTIANO BOCCI, LUCA CHIANTINI

With the notation of the paper, the 5 decompositions of  $T = \lambda_1 \ell_1^7 + \dots + \lambda_{12} \ell_{12}^7 =$

$$\begin{aligned}
&= +2.425782032500251 \cdot 10^2 \cdot (x_0 - 3.831393646843184x_1 + 1.346964775131610 \cdot 10^{-1}x_2)^7 + \\
&\quad +4.146536442894879 \cdot 10^2 \cdot (x_0 + 9.931270838081495 \cdot 10^{-1}x_1 - 6.769701755660390 \cdot 10^{-1}x_2)^7 + \\
&\quad +4.843082801697150 \cdot 10^2 \cdot (x_0 + 3.183385725212400x_1 - 7.633860595893790 \cdot 10^{-1}x_2)^7 + \\
&\quad -3.093559475729942 \cdot 10^1 \cdot (x_0 - 8.878812851871381 \cdot 10^{-1}x_1 + 9.326430222177290 \cdot 10^{-1}x_2)^7 + \\
&\quad +5.913320307260028 \cdot 10^2 \cdot (x_0 - 8.333546205381460 \cdot 10^{-1}x_1 + 4.787791245905811x_2)^7 + \\
&\quad +1.863359371761127 \cdot 10^2 \cdot (x_0 + 1.150535726607133x_1 - 7.356530267574411x_2)^7 + \\
&\quad -6.986594239306317 \cdot 10^2 \cdot (x_0 - 6.33358363820080 \cdot 10^{-1}x_1 + 3.556043275765582x_2)^7 + \\
&\quad +9.082119499105495 \cdot 10^1 \cdot (x_0 + 2.649721933021775x_1 - 2.942789804855117x_2)^7 + \\
&\quad -3.774941091391256 \cdot 10^1 \cdot (x_0 + 9.281823004496396 \cdot 10^{-1}x_1 + 5.416247221839678x_2)^7 + \\
&\quad -8.149598050955672 \cdot 10^{-1} \cdot (x_0 - 3.760716164753004x_1 + 1.290194389580469x_2)^7 + \\
&\quad +5.360726064748198 \cdot (x_0 + 2.159937720250393x_1 - 1.622029661864421x_2)^7 + \\
&\quad -1.967556570270287 \cdot 10^1 \cdot (x_0 - 8.097853608809100 \cdot 10^{-1}x_1 + 5.078077230490563 \cdot 10^{-1}x_2)^7
\end{aligned}$$

are (in each row, the first value denotes the real part and the second one the imaginary part, both expressed in scientific notation; the square brackets identify each linear form):

```

1 (real)
[-3.831393646843184e+00 0.000000000000000e+00
1.346964775131610e-01 0.000000000000000e+00
2.425782032500251e+02 0.000000000000000e+00]
[9.931270838081495e-01 0.000000000000000e+00
-6.769701755660390e-01 0.000000000000000e+00
4.146536442894879e+02 0.000000000000000e+00]
[3.183385725212400e+00 0.000000000000000e+00
-7.633860595893790e-01 0.000000000000000e+00
4.843082801697150e+02 0.000000000000000e+00]
[-8.878812851871381e-01 0.000000000000000e+00
9.326430222177290e-01 0.000000000000000e+00
-3.093559475729942e+01 0.000000000000000e+00]
[-8.333546205381460e-01 0.000000000000000e+00
4.787791245905811e+00 0.000000000000000e+00
5.913320307260028e+02 0.000000000000000e+00]
[1.150535726607133e+00 0.000000000000000e+00
-7.356530267574411e+00 0.000000000000000e+00
1.863359371761127e+02 0.000000000000000e+00]
[-6.33358363820080e-01 0.000000000000000e+00
3.556043275765582e+00 0.000000000000000e+00

```

-6.986594239306317e+02 0.000000000000000e+00]  
 [2.649721933021775e+00 0.000000000000000e+00  
 -2.942789804855117e+00 0.000000000000000e+00  
 9.082119499105495e+01 0.000000000000000e+00]  
 [9.281823004496396e-01 0.000000000000000e+00  
 5.416247221839678e-01 0.000000000000000e+00  
 -3.774941091391256e+01 0.000000000000000e+00]  
 [-3.760716164753004e+00 0.000000000000000e+00  
 1.290194389580469e+00 0.000000000000000e+00  
 -8.149598050955672e-01 0.000000000000000e+00]  
 [2.159937720250393e+00 0.000000000000000e+00  
 -1.622029661864421e+00 0.000000000000000e+00  
 5.360726064748198e+00 0.000000000000000e+00]  
 [-8.097853608809100e-01 0.000000000000000e+00  
 5.078077230490563e-01 0.000000000000000e+00  
 -1.967556570270287e+01 0.000000000000000e+00]

2 (autoconjugate)

[9.735985352499752e-01 -2.385331786692452e-13  
 5.626282630260806e-01 8.970642696552733e-14  
 -3.318025977488983e+01 -1.251329682233626e-11]  
 [3.234937766484757e+00 1.461200015184575e-01  
 -2.171622682249293e+00 -4.991550454977317e-01  
 4.391609208203581e-01 8.163339087845187e-01]  
 [-3.842182004806856e+00 -1.213183199733070e-13  
 1.388281489482307e+00 -3.271642939201014e-13  
 -6.536252037713457e-01 -1.971901916926477e-13]  
 [2.652364549847380e+00 -2.899460185834535e-14  
 -2.938656056108673e+00 4.460407737605365e-14  
 9.190178302429362e+01 2.574121471532465e-12]  
 [3.183084754795606e+00 -8.800469034064842e-16  
 -7.627000581847865e-01 5.271933063710765e-16  
 4.840821321929629e+02 9.002937284563473e-13]  
 [-6.315831748176233e-01 -6.585010314807960e-15  
 3.544233074556528e+00 4.500544902030779e-14  
 -6.944857035908982e+02 -1.380690006769214e-11]  
 [1.150543781376376e+00 1.206174916890124e-17  
 -7.356557226421073e+00 -2.658463726934457e-16  
 1.863328076222213e+02 1.459179999052651e-13]  
 [-9.010153969176740e-01 3.038151327738881e-14  
 7.715147560418783e-01 8.223028378009922e-14  
 -4.706849257611326e+01 -6.495323376376483e-12]  
 [-3.831468955538994e+00 -9.422801081071519e-16  
 1.345668989225407e-01 7.195138311110599e-16  
 2.424848451040679e+02 5.597119989708688e-13]  
 [1.009845150809269e+00 -2.110461870367952e-14  
 -6.950923066399680e-01 3.532374046044673e-14  
 4.121031873724289e+02 9.669723355365534e-12]  
 [-8.340914793360875e-01 2.512286169029099e-15  
 4.792089380347218e+00 -1.373120367409442e-14]

5.851600655456109e+02 2.179001423741056e-11]  
 [3.234937766491346e+00 -1.461200015166160e-01  
 -2.171622682267270e+00 4.991550455070594e-01  
 4.391609207712239e-01 -8.163339087859375e-01]

3 (autoconjugate)

[1.005001612671898e+00 -2.708212343618954e-14  
 -6.598002261381354e-01 -1.554479743710868e-13  
 4.337407534030333e+02 -1.041155772707469e-10]  
 [1.150520895798307e+00 5.696669264781962e-16  
 -7.356423225210541e+00 -4.088743232877334e-15  
 1.863511723269405e+02 -1.447730824111204e-13]  
 [-8.322617395484624e-01 4.055325199312090e-04  
 4.812978091014508e+00 -3.182909721708285e-02  
 3.006652949195586e+02 -2.863875674493717e+02]  
 [-3.830823310430551e+00 2.182997706212664e-14  
 1.346574912471186e-01 -1.341889923830997e-15  
 2.428197801331322e+02 1.205023580919118e-11]  
 [-6.354795085727019e-01 -2.957334897801811e-14  
 3.576719135878232e+00 -1.356084298673177e-13  
 -7.055750205139029e+02 -3.067603115969320e-10]  
 [9.950033344746856e-01 2.846518593752068e-14  
 3.225712374894912e-01 8.762263782385524e-13  
 -5.408408352141774e+01 1.111114845964156e-10]  
 [-8.322617395491898e-01 -4.055325191112392e-04  
 4.812978091015876e+00 3.182909720992971e-02  
 3.006652949674503e+02 2.863875674495862e+02]  
 [3.182569109629301e+00 -2.268909886360415e-15  
 -7.634631750730491e-01 8.921086525753852e-16  
 4.852537489625008e+02 2.706113111372588e-12]  
 [2.646194197122523e+00 5.572799166575493e-15  
 -2.934345730938198e+00 2.019977067557743e-15  
 9.246391644825623e+01 -4.683545218320262e-13]  
 [-8.018716721888144e-01 -1.468812484833881e-12  
 8.736655344150954e-01 -4.181448671472174e-12  
 -5.215979235842930e+01 -3.321032684966418e-11]  
 [-3.724278744828554e+00 6.745860380713564e-13  
 1.287352930852977e+00 -5.101427635358091e-13  
 -8.590795812944648e-01 -1.340336966849237e-12]  
 [-1.951845835469885e+00 -5.027820060244867e-11  
 9.457310260372470e-02 -7.081355145414090e-12  
 -1.726923628323185e+00 1.064730331353826e-10]

4 (conjugate of 5)

[8.871080662294264e-01 -1.518977881643617e-02  
 5.794347285352911e-01 -3.527509780254044e-03  
 -3.784645784302672e+01 -2.233952247823488e+00]  
 [1.150533198612537e+00 -1.261436771425850e-05  
 -7.356511158381491e+00 8.106864172696964e-05  
 1.863384614250756e+02 1.148277808299222e-02]

[-3.734238116895447e+00 2.604802092678453e-02  
 1.294948526537122e+00 -3.978161527330052e-04  
 -8.386848690064069e-01 -2.901054348598004e-02]  
 [3.183693432756871e+00 -1.153606488331249e-04  
 -7.634736896171606e-01 -5.517359658030498e-05  
 4.839948354784190e+02 1.709044875608093e-01]  
 [2.649349855503243e+00 4.695465501664682e-04  
 -2.941405225650593e+00 -8.693376084916177e-04  
 9.115555296555472e+01 -1.981186958414906e-01]  
 [1.970589988565935e+00 -1.613145916033874e-02  
 -1.331743373120136e+00 -1.080808639620336e-01  
 8.708862602469846e+00 -1.997425105237431e-01]  
 [-2.820864216119118e-01 -6.159645655877282e-02  
 -7.135152344183365e-02 -8.403412154774516e-01  
 1.484842925621724e+00 3.721571304249159e+00]  
 [-8.328040294826173e-01 1.097199576145451e-03  
 4.784308720657766e+00 -6.835595653979283e-03  
 5.963328710502550e+02 9.872059117686813e+00]  
 [-6.350231367366657e-01 -2.806118262934982e-03  
 3.565986850409963e+00 1.698159735954104e-02  
 -7.019430820410501e+02 -7.641756372311298e+00]  
 [-8.252421716476096e-01 2.784867326012282e-02  
 8.018082379368519e-01 -2.450075134863612e-02  
 -5.381102212296911e+01 -4.499510946608418e+00]  
 [9.827436116463596e-01 1.343520631299445e-03  
 -6.747014878842543e-01 5.103682294193850e-03  
 4.114194820815013e+02 1.012588211647184e+00]  
 [-3.831416838107858e+00 5.216766393641701e-05  
 1.346802741335904e-01 -1.415381626744476e-05  
 2.425593999046615e+02 1.348541737258003e-02]

5 (conjugate of 4)

[9.827436116398426e-01 -1.343520632010474e-03  
 -6.747014878840080e-01 -5.103682295484001e-03  
 4.114194820794906e+02 -1.012588210938004e+00]  
 [8.871080662099992e-01 1.518977881688473e-02  
 5.794347285500229e-01 3.527509779870179e-03  
 -3.784645784325789e+01 2.233952247935992e+00]  
 [-6.350231367382669e-01 2.806118264202153e-03  
 3.565986850419772e+00 -1.698159736720311e-02  
 -7.019430820447103e+02 7.641756376690111e+00]  
 [1.150533198612533e+00 1.261436772284489e-05  
 -7.356511158381470e+00 -8.106864178502606e-05  
 1.863384614250798e+02 -1.148277809222015e-02]  
 [-3.734238116880985e+00 -2.604802092667942e-02  
 1.294948526538293e+00 3.978161555615296e-04  
 -8.386848690208246e-01 2.901054348951974e-02]  
 [-8.328040294820309e-01 -1.097199576704867e-03  
 4.784308720654153e+00 6.835595657467825e-03  
 5.963328710554332e+02 -9.872059122757552e+00]

```
[2.649349855502912e+00 -4.695465500843529e-04
-2.941405225649718e+00 8.693376082392249e-04
9.115555296574394e+01 1.981186957798591e-01]
[-2.820864213412536e-01 6.159645651486255e-02
-7.135152378024824e-02 8.403412158629966e-01
1.484842926138330e+00 -3.721571302830541e+00]
[1.970589988481377e+00 1.613145918701866e-02
-1.331743372964694e+00 1.080808639390329e-01
8.708862604845381e+00 1.997425104523145e-01]
[-8.252421716304489e-01 -2.784867325569348e-02
8.018082379286424e-01 2.450075134018378e-02
-5.381102212508967e+01 4.499510945255777e+00]
[3.183693432757071e+00 1.153606488763884e-04
-7.634736896172011e-01 5.517359658234946e-05
4.839948354782084e+02 -1.709044876215579e-01]
[-3.831416838107870e+00 -5.216766393655687e-05
1.346802741335821e-01 1.415381626129550e-05
2.425593999046545e+02 -1.348541737633437e-02]
```

With the notation of the paper, the 16 decompositions of  $T = \lambda_1 \ell_1^8 + \dots + \lambda_{15} \ell_{15}^8 =$

$$\begin{aligned}
&= +3.802256643629860 \cdot (x_0 - 8.917867308121220 \cdot 10^{-1}x_1 - 3.882527532557760 \cdot 10^{-1}x_2)^8 + \\
&\quad +4.499965370038940 \cdot 10^1 \cdot (x_0 + 8.752472902826010 \cdot 10^{-1}x_1 - 5.012502093548760 \cdot 10^{-1}x_2)^8 + \\
&\quad -5.411549110491870 \cdot 10^1 \cdot (x_0 + 7.119541680224431 \cdot 10^{-1}x_1 - 4.656057771083370 \cdot 10^{-2}x_2)^8 + \\
&\quad -3.750700782420560 \cdot 10^1 \cdot (x_0 - 6.257070109519970 \cdot 10^{-1}x_1 + 2.294191400826210 \cdot 10^{-1}x_2)^8 + \\
&\quad -9.252016941613800 \cdot 10^1 \cdot (x_0 + 8.830647057133760 \cdot 10^{-1}x_1 - 5.026318665541210 \cdot 10^{-1}x_2)^8 + \\
&\quad -7.436378620768880 \cdot (x_0 + 8.662890126034720 \cdot 10^{-1}x_1 - 7.498635837727520 \cdot 10^{-1}x_2)^8 + \\
&\quad +7.366967625095110 \cdot (x_0 - 5.037776998327460 \cdot 10^{-1}x_1 + 7.225195917485460 \cdot 10^{-1}x_2)^8 + \\
&\quad -4.554394894892720 \cdot (x_0 + 9.363491701837950 \cdot 10^{-1}x_1 - 3.075057135421950 \cdot 10^{-1}x_2)^8 + \\
&\quad +1.637407925571110 \cdot (x_0 + 3.901539106331100 \cdot 10^{-1}x_1 + 3.211377682018530 \cdot 10^{-1}x_2)^8 + \\
&\quad +6.417745789016570 \cdot (x_0 + 7.404821190992460 \cdot 10^{-1}x_1 - 7.815152102127080 \cdot 10^{-1}x_2)^8 + \\
&\quad -9.944247658494602 \cdot (x_0 - 5.295293887908490 \cdot 10^{-1}x_1 - 5.561058003667060 \cdot 10^{-1}x_2)^8 + \\
&\quad +9.841403826077800 \cdot (x_0 - 5.708459618609850 \cdot 10^{-1}x_1 + 6.892129936226110 \cdot 10^{-1}x_2)^8 + \\
&\quad -7.433335437717520 \cdot (x_0 - 9.352316331313800 \cdot 10^{-1}x_1 + 8.462494124044420 \cdot 10^{-1}x_2)^8 + \\
&\quad +1.417745789016570 \cdot (x_0 - 3.476378206768880 \cdot 10^{-1}x_1 - 8.815152102127080 \cdot 10^{-1}x_2)^8 + \\
&\quad -9.044247658494601 \cdot (x_0 - 4.295293887908490 \cdot 10^{-1}x_1 - 5.061058003667061 \cdot 10^{-1}x_2)^8
\end{aligned}$$

are (in each row, the first value denotes the real part and the second one the imaginary part, both expressed in scientific notation; the square brackets identify each linear form):

```

1 (real)
[-8.917867308121220e-01 0.000000000000000e+00
-3.882527532557760e-01 0.000000000000000e+00
3.802256643629860e+00 0.000000000000000e+00]
[8.752472902826010e-01 0.000000000000000e+00
-5.012502093548760e-01 0.000000000000000e+00
4.499965370038940e+01 0.000000000000000e+00]
[7.119541680224431e-01 0.000000000000000e+00
-4.656057771083370e-02 0.000000000000000e+00
-5.411549110491870e+01 0.000000000000000e+00]
[-6.257070109519970e-01 0.000000000000000e+00
2.294191400826210e-01 0.000000000000000e+00
-3.750700782420560e+01 0.000000000000000e+00]
[8.830647057133760e-01 0.000000000000000e+00
-5.026318665541210e-01 0.000000000000000e+00
-9.252016941613800e+01 0.000000000000000e+00]
[8.662890126034720e-01 0.000000000000000e+00
-7.498635837727520e-01 0.000000000000000e+00
-7.436378620768880e+00 0.000000000000000e+00]
[-5.037776998327460e-01 0.000000000000000e+00
7.225195917485460e-01 0.000000000000000e+00
7.366967625095110e+00 0.000000000000000e+00]
[9.363491701837950e-01 0.000000000000000e+00
-3.075057135421950e-01 0.000000000000000e+00
-4.554394894892720e+00 0.000000000000000e+00]
[3.901539106331100e-01 0.000000000000000e+00
3.211377682018530e-01 0.000000000000000e+00
1.637407925571110e+00 0.000000000000000e+00]
[7.404821190992460e-01 0.000000000000000e+00
-7.815152102127080e-01 0.000000000000000e+00
6.417745789016570e+00 0.000000000000000e+00]
[-5.295293887908490e-01 0.000000000000000e+00
-5.561058003667060e-01 0.000000000000000e+00
-9.944247658494602e+00 0.000000000000000e+00]
[-5.708459618609850e-01 0.000000000000000e+00
6.892129936226110e-01 0.000000000000000e+00
9.841403826077800e+00 0.000000000000000e+00]
[-9.352316331313800e-01 0.000000000000000e+00
8.462494124044420e-01 0.000000000000000e+00
-7.43335437717520e+00 0.000000000000000e+00]
[-3.476378206768880e-01 0.000000000000000e+00
-8.815152102127080e-01 0.000000000000000e+00
1.417745789016570e+00 0.000000000000000e+00]
[-4.295293887908490e-01 0.000000000000000e+00
-5.061058003667061e-01 0.000000000000000e+00
-9.044247658494601e+00 0.000000000000000e+00]

```

```

2 (conjugate of 4)
[7.210246592096185e-01 5.587182013586815e-02
-7.866570924057401e-01 6.875331926570877e-03]

```

3.566957614769288e+00 2.182210446207240e+00]  
 [-5.359270991455427e-01 2.164606001277306e-02  
 -5.547304260284033e-01 -1.177478307916202e-02  
 -9.196662499420281e+00 -6.400883938428257e-01]  
 [-9.350551897828314e-01 -4.408853547054836e-04  
 8.462648024313514e-01 1.215947567002245e-04  
 -7.440993624681908e+00 2.494497689814429e-02]  
 [-4.298652919192623e-01 -6.815420557929105e-03  
 -5.124775322398207e-01 1.140881631001146e-02  
 -9.745542667162736e+00 7.624086322255483e-01]  
 [-6.255988358991727e-01 -9.500935939905266e-05  
 2.289428665769234e-01 6.764564024817357e-04  
 -3.748725648423427e+01 -1.367460178425555e-02]  
 [7.132860636915525e-01 -5.394305970591783e-03  
 -4.659341042895759e-02 5.908481044879016e-03  
 -5.756444596616613e+01 1.424446594059909e+00]  
 [7.847544757787565e-01 -1.448689966219596e-01  
 -9.670557676087353e-02 1.693171805263438e-01  
 1.363421513653543e+00 -1.631298941107974e+00]  
 [-4.868981030765320e-01 -2.400720965946428e-02  
 7.301757390244913e-01 -5.339910821843638e-03  
 3.529603037494539e+00 2.287019780434973e+00]  
 [4.146668732470665e-01 -1.296328541577055e-02  
 2.954404435570108e-01 9.901000576687094e-03  
 2.044672705325320e+00 -3.623109951564241e-02]  
 [8.804221545196037e-01 -4.346805217191824e-02  
 -7.469480079852904e-01 -1.857330587837774e-02  
 -4.555520810334770e+00 -2.081789686858791e+00]  
 [-3.475611164228027e-01 -2.059330410124636e-03  
 -8.837159048278909e-01 6.054185006028804e-03  
 1.371500720139498e+00 1.029017307810875e-01]  
 [9.674964104295630e-01 2.810613840999488e-02  
 -3.335899173358525e-01 -5.489487521096994e-02  
 -2.332331194169219e+00 1.920762538122402e-01]  
 [-5.591671811118130e-01 -5.926107389426834e-03  
 6.973843510970794e-01 -5.160329091032791e-03  
 1.364525554349997e+01 -2.265361144203229e+00]  
 [8.914815551059837e-01 1.949209047857059e-05  
 -5.031129333617723e-01 2.913586414177898e-04  
 -4.809237085470810e+01 -7.827333843930383e-02]  
 [-8.909197149661484e-01 -5.961238631853069e-03  
 -3.889115901250618e-01 2.874498244890146e-03  
 3.821621649161002e+00 -2.292912086670982e-01]

3 (autoconjugate)

[-9.453727247365973e-01 6.126490374042115e-14  
 8.517295407301952e-01 -1.359890390399687e-14  
 -6.787722743380753e+00 -4.165216348911427e-12]  
 [-5.460177451549906e-01 2.451823866162245e-01  
 6.478331274052218e-01 -1.568219289657023e-01

4.266434663995381e-01 -7.515413318420704e-02]  
 [7.242510275857044e-01 8.901028785562870e-15  
 -6.138374599134590e-02 -1.705890982672039e-14  
 -5.627630310127955e+01 -9.448154064672920e-13]  
 [-4.814757292341366e-01 9.063185349513528e-02  
 -5.260311512905227e-01 -6.649260460054320e-02  
 -8.450735284174789e+00 1.076403912127062e+00]  
 [-3.278538973742860e-01 4.271390641359674e-14  
 -9.216379714395625e-01 -3.129153837086451e-14  
 9.084241699895901e-01 -1.929301987266263e-13]  
 [2.584441485527262e-01 -5.474013440882192e-13  
 4.484517146692124e-01 4.442742153982701e-13  
 7.750431137402102e-01 -1.114896450984601e-12]  
 [8.110586370620925e-01 2.437644641644411e-01  
 -8.210008330210390e-01 2.014478541212550e-02  
 2.132659961529320e-01 9.93355272138112e-01]  
 [-6.258152397698858e-01 -4.142790711175737e-15  
 2.259448495111051e-01 -9.519335732004197e-15  
 -3.746731302097189e+01 8.055292544106862e-13]  
 [8.944009272073485e-01 9.113911882130399e-15  
 -5.114565760784248e-01 -2.156574344016476e-14  
 -4.910316134956280e+01 -2.591588402212075e-12]  
 [-4.814757292343216e-01 -9.063185349578860e-02  
 -5.260311512905305e-01 6.649260460101844e-02  
 -8.450735284110136e+00 -1.076403912127466e+00]  
 [-5.345445809250391e-01 -1.668554888440560e-13  
 7.094871903266680e-01 1.472578298449684e-14  
 1.537628706014148e+01 2.314718989399056e-11]  
 [1.030057912274576e+00 -9.003540100971375e-15  
 -4.064821505690595e-01 2.737534049272738e-13  
 -1.531144336099343e+00 2.592701986263435e-12]  
 [8.110586370616590e-01 -2.437644641648224e-01  
 -8.210008330212978e-01 -2.014478541209450e-02  
 2.132659961548521e-01 -9.93355272111755e-01]  
 [-9.303024577575947e-01 4.235183709809520e-14  
 -3.730730306574108e-01 -3.631805549656961e-14  
 2.655450533767568e+00 5.976416193528844e-13]  
 [-5.460177451527439e-01 -2.451823866163033e-01  
 6.478331274026510e-01 1.568219289659575e-01  
 4.266434663988772e-01 7.515413316384172e-02]

4 (conjugate of 2)

[-4.298652919192762e-01 6.815420558799390e-03  
 -5.124775322404064e-01 -1.140881631168013e-02  
 -9.745542667201839e+00 -7.624086323605784e-01]  
 [-4.868981030748857e-01 2.400720966457264e-02  
 7.301757390258910e-01 5.339910822903982e-03  
 3.529603036935649e+00 -2.287019780623562e+00]  
 [-5.359270991451139e-01 -2.164606001626799e-02  
 -5.547304260286808e-01 1.177478308094900e-02]



-9.196662499357597e+00 6.400883939587667e-01]  
 [7.210246592094818e-01 -5.587182014202050e-02  
 -7.866570924061832e-01 -6.875331927427410e-03  
 3.566957614549039e+00 -2.182210446285172e+00]  
 [-8.909197149663994e-01 5.961238632794111e-03  
 -3.889115901249647e-01 -2.874498245356277e-03  
 3.821621649147228e+00 2.292912087016949e-01]  
 [7.847544757197836e-01 1.448689966432378e-01  
 -9.670557669182169e-02 -1.693171805336232e-01  
 1.363421515363791e+00 1.631298939786447e+00]  
 [-6.255988358991604e-01 9.500935941172888e-05  
 2.289428665768626e-01 -6.764564025764381e-04  
 -3.748725648423138e+01 1.367460178604349e-02]  
 [8.914815551059431e-01 -1.949209044527232e-05  
 -5.031129333616252e-01 -2.913586413623247e-04  
 -4.809237085469305e+01 7.827333840745980e-02]  
 [7.132860636938447e-01 5.394305971286913e-03  
 -4.659341043117667e-02 -5.908481045936540e-03  
 -5.756444596781816e+01 -1.424446592551595e+00]  
 [8.804221545202190e-01 4.346805217576268e-02  
 -7.469480079853921e-01 1.857330588002622e-02  
 -4.555520810124364e+00 2.081789686935680e+00]  
 [-5.591671811103230e-01 5.926107389821237e-03  
 6.973843510980702e-01 5.160329091467180e-03  
 1.364525554405268e+01 2.265361144391191e+00]  
 [-3.475611164227918e-01 2.059330410387417e-03  
 -8.837159048281190e-01 -6.054185006909320e-03  
 1.371500720133891e+00 -1.029017307958664e-01]  
 [4.146668732510270e-01 1.296328541926080e-02  
 2.954404435524577e-01 -9.901000579248757e-03  
 2.044672705431295e+00 3.623109952243653e-02]  
 [-9.350551897828143e-01 4.408853548091634e-04  
 8.462648024313597e-01 -1.215947567306519e-04  
 -7.440993624682475e+00 -2.494497690410307e-02]  
 [9.674964104265793e-01 -2.810613841175236e-02  
 -3.335899173324060e-01 5.489487521103795e-02  
 -2.332331194338878e+00 -1.920762539688517e-01]

5 (autoconjugate)

[6.258544940438240e-01 2.444195019990492e-13  
 -7.678349426672247e-01 2.837687767057173e-13  
 1.244939234000623e+00 -1.997444473277737e-12]  
 [-9.401405160633410e-01 5.120253179780043e-15  
 8.486645547434080e-01 -1.448006211463015e-15  
 -7.119934452520422e+00 -2.942474822825725e-13]  
 [-5.327857001978194e-01 -9.946023496985867e-15  
 7.042098767748363e-01 3.864530223607332e-15  
 1.661725817624452e+01 9.214851104388799e-14]  
 [-8.058836626915773e-03 -3.117165640023525e-13  
 3.239010202815472e-01 -1.022829417733975e-13]

-2.433110865372195e-01 3.347956609753115e-13]  
 [-6.254611053056876e-01 -6.865710257264457e-17  
 2.237779292511124e-01 2.415670202933484e-16  
 -3.745411741688740e+01 2.396173537366764e-14]  
 [2.319049584348891e-01 -4.877214355037546e-14  
 4.734759282157470e-01 2.577521258494836e-14  
 6.857137110583185e-01 -3.911909858544949e-15]  
 [-3.174799314714942e-01 -6.092877396189633e-15  
 -9.497515810221587e-01 -9.987833043262340e-15  
 6.699239016539020e-01 -1.049809111169919e-13]  
 [7.259253023514881e-01 -5.287626890157493e-15  
 -6.335624566560175e-02 3.831138490760673e-15  
 -5.650897239858197e+01 9.512998028204933e-13]  
 [8.951793421099928e-01 -6.385706850450812e-15  
 -5.138988210434815e-01 -9.012362796149975e-15  
 -4.942304375858109e+01 7.667564499991286e-13]  
 [-4.667153710418027e-01 -7.103926301118253e-02  
 -5.401295115839617e-01 7.968158826996549e-02  
 -8.473755277891890e+00 8.844434656999308e-01]  
 [-9.183491416254729e-01 7.234149260529343e-15  
 -3.771658688987371e-01 -2.996572174424061e-15  
 2.970660659221281e+00 1.624521914558863e-13]  
 [8.931840905959586e-01 2.783805681948367e-01  
 -8.508981986685611e-01 4.430143733663597e-02  
 -1.381558755805500e-01 4.409621335978645e-01]  
 [1.045340315299355e+00 -2.250518293858000e-13  
 -4.247877586914204e-01 1.915246932403247e-13  
 -1.287385578972456e+00 -3.067680224427827e-12]  
 [-4.667153710418070e-01 7.103926301123123e-02  
 -5.401295115839588e-01 -7.968158827002864e-02  
 -8.473755277884063e+00 -8.844434656998415e-01]  
 [8.931840905955270e-01 -2.783805681958071e-01  
 -8.508981986688241e-01 -4.430143733662183e-02  
 -1.381558755757902e-01 -4.409621335948596e-01]

6 (autoconjugate)

[-6.255385703387918e-01 -1.444725144638531e-14  
 2.283469024719451e-01 1.043006081350752e-13  
 -3.748514540129286e+01 -1.473578203903259e-12]  
 [-8.781283057804598e-01 -2.736729625470863e-12  
 -3.948140098598941e-01 1.290519137408554e-12  
 4.398514704190381e+00 -1.360723992250429e-10]  
 [6.120109926509152e-01 1.838538128435142e-11  
 -7.912586545235696e-01 2.533985933410310e-13  
 2.366081266062438e+00 1.752635498753277e-10]  
 [9.775738713979871e-01 -2.196149620665999e-12  
 -3.719513431180045e-01 2.918034452850486e-12  
 -4.230689651287308e+00 -1.447177545984765e-10]  
 [-3.446982072055478e-01 -3.616656534801907e-13  
 -8.909616771375186e-01 1.068000939422054e-12]

1.261359921878165e+00 1.638458872700241e-11]  
 [-5.758302741303548e-01 8.159382200380490e-12  
 -5.331791881908783e-01 -3.970043301808161e-12  
 -8.819892202090991e+00 -7.156417559245343e-11]  
 [7.136475953007034e-01 -1.976323835486959e-13  
 -4.802791096534909e-02 1.981835631340674e-13  
 -5.501773217349667e+01 6.945440750305565e-11]  
 [8.919277691291594e-01 -1.015601990526915e-14  
 -5.039093459997603e-01 9.435838612195657e-15  
 -4.833818646087219e+01 5.687906742823934e-13]  
 [-4.699112260037994e-01 -4.091854893112368e-12  
 7.297670428547317e-01 -5.310622953761182e-13  
 3.230108988119738e+00 2.687457223990788e-10]  
 [1.004649199454523e+00 -4.574700386174848e-02  
 -6.694665281882186e-01 -7.271646765862327e-02  
 -9.857441814950940e-01 2.311468999311459e+00]  
 [-9.347041097843259e-01 -7.057253544572040e-14  
 8.461346026233205e-01 1.715524966007520e-14  
 -7.461596653054906e+00 3.802585633524980e-12]  
 [-4.177035341370876e-01 -1.783649955706436e-12  
 -5.262701472629219e-01 2.330249220579977e-12  
 -1.063645993535626e+01 2.025370043120395e-10]  
 [4.033622271207074e-01 -7.851456572567639e-13  
 3.098405515235254e-01 5.841696280894405e-13  
 1.700515056728862e+00 1.357217181523207e-12]  
 [1.004649199488716e+00 4.574700384587309e-02  
 -6.694665281474307e-01 7.271646768188497e-02  
 -9.857441792789304e-01 -2.311468999429995e+00]  
 [-5.585261356956531e-01 -7.647436828760179e-13  
 6.988843263735568e-01 -6.157744263492540e-13  
 1.393251958441143e+01 -2.657463147107131e-10]

7 (conjugate of 14)

[-6.245418856021472e-01 2.396242989086739e-04  
 2.204039424912613e-01 -1.277403194764817e-02  
 -3.613644777438486e+01 -8.060940289245340e-01]  
 [-4.614020553281961e-01 -3.773773538116904e-02  
 -6.278347868110032e-01 4.251037664972397e-02  
 -8.544985343930705e+00 4.238461475451734e+00]  
 [-3.647461364566319e-01 2.475631674663658e-02  
 -8.506455517711713e-01 -6.544641081002449e-02  
 1.179807352428393e+00 -1.559059183396279e+00]  
 [8.925137465232057e-01 3.853344295723471e-04  
 -5.061567882195200e-01 -4.901520505690420e-04  
 -4.841570038935597e+01 -1.817311564774030e-01]  
 [3.354032712746878e-01 -3.839074295146552e-03  
 3.797034011295609e-01 5.043789914147877e-03  
 1.095965811476493e+00 -4.855078128448288e-02]  
 [-4.696650194009023e-01 2.824603317701370e-02  
 -4.822604572627292e-01 -7.315078891522681e-02

-9.661702837570505e+00 -2.140366033594888e+00]  
 [8.278772533423157e-01 1.232301854875163e-01  
 -7.816330522994717e-01 2.610950675276983e-02  
 -5.156782959930861e-01 2.696736260830602e+00]  
 [7.190623422704341e-01 -5.209831728056452e-05  
 -5.481170627822687e-02 -1.594960169592214e-04  
 -5.533590827504817e+01 6.497817152074534e-02]  
 [-9.388894938234098e-01 9.363491109448312e-04  
 8.479485856457857e-01 -8.130430692816708e-05  
 -7.183770940792492e+00 -5.232433246136874e-02]  
 [-3.442425827631582e-01 -3.506713457251272e-02  
 5.613067827448105e-01 -4.233475001354453e-02  
 -5.079249888484747e-01 1.744256126899347e-01]  
 [-5.304659519957118e-01 -3.312675590168370e-03  
 7.044956246120507e-01 1.910253193389022e-03  
 1.677227295969116e+01 -2.589541409606139e-01]  
 [9.800626946753164e-01 -4.730303044087445e-03  
 -3.545152727930547e-01 1.393915820485883e-02  
 -2.587834666772369e+00 7.007338478804999e-02]  
 [-9.064590360801259e-01 3.247602762746284e-03  
 -3.820358825972275e-01 -1.927146598614507e-03  
 3.300888201191362e+00 9.206613579416331e-02]  
 [-6.742116809375618e-01 -1.336807241954588e-02  
 2.754575529541676e-01 2.939105367697752e-01  
 -6.673025559306993e-01 3.120559830781826e-01]  
 [7.993117848185278e-01 -1.337000802760138e-01  
 -7.904881554467492e-01 -2.640723811621034e-02  
 1.362304270057196e-01 -2.601717367053863e+00]

8 (autoconjugate)

[7.335719075211914e-01 -1.023051116749458e-12  
 -6.954269212815378e-02 8.343009747955547e-13  
 -5.636536783278187e+01 -1.757391471929326e-10]  
 [-4.667920503673446e-01 6.541545844084905e-02  
 -5.309192050656313e-01 -7.781469005142490e-02  
 -8.431351643834137e+00 5.981232800968304e-01]  
 [-3.180421394812981e-01 2.122837191133927e-13  
 -9.471569788316445e-01 -4.390264193854243e-13  
 6.934148136973352e-01 -3.609039262374939e-12]  
 [2.866265073059403e+00 -9.952369182298325e-01  
 -1.696850901917871e+00 -6.880945487163324e-01  
 2.108105525044448e-06 3.743718113678928e-05]  
 [2.866265073838187e+00 9.952369164276804e-01  
 -1.696850901502247e+00 6.880945496941597e-01  
 2.108105724706816e-06 -3.743718112172383e-05]  
 [1.050324822734379e+00 8.407806284418777e-12  
 -7.206883117568471e-01 8.143410824953869e-12  
 -1.187799288386138e+00 -8.054214128863473e-12]  
 [2.493019153106642e-01 -1.522163705437772e-12  
 4.705170265366122e-01 2.398416040153960e-13

6.039752670637097e-01 7.452109276071071e-12]  
 [-9.499723892261021e-01 1.973981741953956e-12  
 8.517949946501949e-01 -6.258567340593213e-13  
 -6.624825174878012e+00 -8.960422811718494e-11]  
 [2.851420872251650e-01 -3.492798680795504e-11  
 2.269479682857460e-01 1.767475778738793e-11  
 -1.156659663910487e+00 2.159782058058779e-10]  
 [5.252333088484834e-01 4.247837816223491e-12  
 -7.888965781246231e-01 2.636884037943849e-13  
 1.805189181702209e+00 -4.293627825784248e-11]  
 [-5.182736269284077e-01 -2.440786833849415e-12  
 6.986381308732287e-01 9.405350643817458e-13  
 1.631711587426659e+01 6.675708672920083e-11]  
 [-6.254279060262763e-01 -2.358668273715059e-15  
 2.237227119893685e-01 8.239226697280035e-15  
 -3.746755558355696e+01 1.355573639449936e-12]  
 [-9.355620701525017e-01 3.393076462431411e-12  
 -3.689565193109540e-01 -1.642810917818838e-12  
 2.662246490629536e+00 5.328458599915611e-11]  
 [8.956708290787703e-01 -5.428302122037487e-15  
 -5.130671070286414e-01 -2.559491653992760e-14  
 -4.948912632875481e+01 1.027608987486106e-12]  
 [-4.667920503652526e-01 -6.541545844102810e-02  
 -5.309192050665471e-01 7.781469004852273e-02  
 -8.431351644302383e+00 -5.981232801227627e-01]

9 (conjugate of 11)

[2.618631896157466e-01 -4.120004497905725e-02  
 4.484555219280904e-01 4.016094624416294e-02  
 7.586388844277393e-01 -1.551201921798171e-01]  
 [1.017572065992218e+00 2.745803914232527e-02  
 -3.963759722114385e-01 -2.657533685793061e-02  
 -1.630244334018100e+00 5.293407518358932e-01]  
 [-1.608979957465187e-01 1.480149559990506e-01  
 4.214860868252717e-01 -1.182082271323576e-01  
 -2.244636675010166e-01 8.654147668341043e-02]  
 [-5.325037132844614e-01 -1.420043658460196e-03  
 7.038961351793622e-01 3.381242835063800e-04  
 1.665329757459413e+01 -6.952006098344651e-02]  
 [-8.069797694089559e-01 -1.043444965497151e+00  
 2.220700097308438e+00 2.636358899825566e-01  
 9.702382886369641e-06 1.273937356028570e-06]  
 [7.239969214094059e-01 2.480246945274947e-03  
 -6.093588243487003e-02 -2.976746909749506e-03  
 -5.611964087069541e+01 -3.686471926309850e-01]  
 [-3.282107730945046e-01 -7.894788409362025e-03  
 -9.197036145228337e-01 1.775292416137365e-02  
 8.989739709235816e-01 1.743098380124352e-01]  
 [8.939680479397665e-01 9.630273588788418e-04  
 -5.103252949703556e-01 -1.837770031770692e-03]

-4.896257775587133e+01 -2.926538613773213e-01]  
 [-9.184163307969639e-01 -8.814540143221184e-03  
 -3.775067980836966e-01 3.145036000917542e-03  
 2.943780721739422e+00 -2.423358355158789e-01]  
 [-4.931178467089601e-01 6.855987991361819e-02  
 -5.372916212744960e-01 -6.320111582519758e-02  
 -9.517984583898024e+00 8.164168170719230e-01]  
 [8.594191895339430e-01 -2.070316213832543e-01  
 -8.134639030643139e-01 -4.060195407572972e-02  
 -3.176677959005466e-01 -1.110375909474046e+00]  
 [7.682971684799020e-01 1.989596000585541e-01  
 -8.050728608684159e-01 1.217455892473982e-02  
 6.255861669396831e-01 1.372475526561244e+00]  
 [-4.640514597062149e-01 -8.060271985802775e-02  
 -5.162301261261831e-01 7.203789574464939e-02  
 -7.667754980833529e+00 -7.825371889912728e-01]  
 [-6.256520531440247e-01 -1.360232835130338e-04  
 2.244938110044726e-01 1.186899558748021e-03  
 -3.739255294676313e+01 3.538195508996854e-02]  
 [-9.400519843872387e-01 -1.754721325053753e-04  
 8.486430369086068e-01 2.723784975440596e-04  
 -7.119491402360589e+00 6.722601960541419e-03]

10 (conjugate of 13)

[9.317930943226062e-01 -1.472234491764690e-01  
 -8.619742514352065e-01 -7.025631107381143e-02  
 -9.898578441358703e-02 -1.187108351476284e-01]  
 [-5.269519643850231e-01 6.933882120761792e-05  
 -5.560628450599662e-01 1.401508804515179e-03  
 -1.027656515093699e+01 -2.132593095701368e-01]  
 [8.513751668923720e-01 3.887048848258774e-02  
 -7.614121528390214e-01 2.510696629578781e-02  
 -5.302412002411908e+00 2.338243159051923e+00]  
 [9.394960875317836e-01 -2.129394015733528e-04  
 -3.043356384837974e-01 -3.837627366862530e-04  
 -3.921664398360300e+00 -3.495708093345942e-02]  
 [8.919571864211547e-01 -3.982251035855760e-04  
 -5.068547905990521e-01 1.975300156667523e-03  
 -4.828796369512096e+01 4.574428254570898e-01]  
 [-3.474138835827502e-01 6.387490854469481e-04  
 -8.813377675335571e-01 -7.829948760551650e-04  
 1.422319245770136e+00 -1.142150474028159e-02]  
 [-4.282634374642520e-01 2.223871485497872e-03  
 -5.040306222168164e-01 9.651758636705505e-06  
 -8.710731695520272e+00 2.119998660182310e-01]  
 [-5.860592500001232e-01 -2.210171003762181e-03  
 6.776996385502782e-01 -1.233879864871571e-03  
 6.127564458191140e+00 -3.187939701195209e-01]  
 [3.577872337677870e-01 4.156190717032709e-03  
 3.514127411437442e-01 -3.256353441593383e-03]

1.353433982496482e+00 2.989672078027166e-02]  
 [-9.352532350831598e-01 -6.157831909051621e-06  
 8.462267205937498e-01 -1.501889115311929e-05  
 -7.433266615921304e+00 -4.353307493020053e-04]  
 [7.144335694866425e-01 -3.378160379662137e-04  
 -4.998816961976084e-02 5.489802762788576e-04  
 -5.439261982638456e+01 8.198220542482362e-02]  
 [-8.921446010558835e-01 2.315794284849591e-04  
 -3.879777515082027e-01 1.386521067725951e-06  
 3.788789374191011e+00 9.467279986091736e-03]  
 [7.392493515531506e-01 -2.799150198383169e-02  
 -7.773940555780661e-01 9.409996851565191e-04  
 5.089666486550386e+00 -2.751465428108128e+00]  
 [-5.187319623393681e-01 -7.483489981751693e-04  
 7.169952569703204e-01 -5.192950714337775e-04  
 1.110016872164469e+01 3.229885745120180e-01]  
 [-6.257960072923841e-01 -2.238575872916590e-05  
 2.296962485959956e-01 1.038913192892972e-05  
 -3.752982441660823e+01 -2.977171861990171e-03]

11 (conjugate of 9)

[-4.931178467087196e-01 -6.855987991289235e-02  
 -5.372916212735263e-01 6.320111582500707e-02  
 -9.517984583986625e+00 -8.164168171533239e-01]  
 [7.682971684817247e-01 -1.989596000590475e-01  
 -8.050728608685467e-01 -1.217455892479434e-02  
 6.255861669209913e-01 -1.372475526558725e+00]  
 [8.594191895310401e-01 2.070316213845736e-01  
 -8.134639030649199e-01 4.060195407460206e-02  
 -3.176677958706943e-01 1.110375909478795e+00]  
 [-1.608979957458642e-01 -1.480149559946564e-01  
 4.214860868228315e-01 1.182082271327070e-01  
 -2.244636674989798e-01 -8.654147668435426e-02]  
 [-9.400519843872076e-01 1.754721324474218e-04  
 8.486430369086069e-01 -2.723784975327942e-04  
 -7.119491402362344e+00 -6.722601957571189e-03]  
 [7.239969214094716e-01 -2.480246945171011e-03  
 -6.093588243496224e-02 2.976746909638158e-03  
 -5.611964087070181e+01 3.686471926165056e-01]  
 [2.618631896137417e-01 4.120004497808183e-02  
 4.484555219300412e-01 -4.016094624323371e-02  
 7.586388844214623e-01 1.551201921749128e-01]  
 [-9.184163307971054e-01 8.814540142830044e-03  
 -3.775067980836644e-01 -3.145036000708681e-03  
 2.943780721736339e+00 2.423358355060330e-01]  
 [-8.069797693364689e-01 1.043444965561910e+00  
 2.220700097327337e+00 -2.636358901841455e-01  
 9.702382884878826e-06 -1.273937348682935e-06]  
 [8.939680479397859e-01 -9.630273588669878e-04  
 -5.103252949704600e-01 1.837770031730070e-03]

-4.896257775587598e+01 2.926538613730037e-01]  
 [-4.640514597077698e-01 8.060271985924424e-02  
 -5.162301261255538e-01 -7.203789574585603e-02  
 -7.667754980730839e+00 7.825371890780009e-01]  
 [1.017572065992693e+00 -2.745803914116343e-02  
 -3.963759722118921e-01 2.657533685599560e-02  
 -1.630244334012974e+00 -5.293407518201476e-01]  
 [-5.325037132845544e-01 1.420043658510465e-03  
 7.038961351793993e-01 -3.381242835766000e-04  
 1.665329757459228e+01 6.952006098343745e-02]  
 [-3.282107730939418e-01 7.894788409181534e-03  
 -9.197036145236675e-01 -1.775292416121190e-02  
 8.989739709171594e-01 -1.743098380089187e-01]  
 [-6.256520531440362e-01 1.360232835198165e-04  
 2.244938110044396e-01 -1.186899558684281e-03  
 -3.739255294676511e+01 -3.538195509029508e-02]

12 (autoconjugate)

[-3.359964856363148e-01 6.284775082082347e-14  
 -9.115956659094101e-01 -1.028173179191613e-13  
 1.000557244123948e+00 -1.298304224003032e-12]  
 [-6.993046429967424e-02 -1.343015071660856e-11  
 4.374667641606872e-01 6.391732995203285e-12  
 -8.984692762365744e-01 -8.181080135170535e-12]  
 [-9.495512172366581e-01 1.738420198809168e-13  
 8.517025569590508e-01 -4.947217223556788e-14  
 -6.616225746425354e+00 -6.890938666036239e-12]  
 [-3.762247261777357e-01 -1.190727523317750e-01  
 -5.773366278117874e-01 5.491438327712161e-02  
 -8.005171739216824e+00 6.779433563239184e+00]  
 [-3.762247261774802e-01 1.19072752322546e-01  
 -5.773366278104883e-01 -5.491438327373667e-02  
 -8.005171739911058e+00 -6.779433563290227e+00]  
 [-5.599670836989721e-01 3.796828675843144e-12  
 5.556288320812062e-01 6.379148701244827e-12  
 1.238898597353144e+00 4.529710693991149e-11]  
 [8.939419952436755e-01 -2.255370911731502e-14  
 -5.088875706053538e-01 3.588687506883570e-14  
 -4.901295480999227e+01 7.287586333004636e-12]  
 [-9.698589722743594e-01 2.012799337467765e-12  
 -3.524240021606473e-01 -9.775575395823064e-13  
 2.014579677034499e+00 2.680465840065004e-11]  
 [8.387448112427448e-01 -5.620028688969319e-01  
 -9.123969777098427e-01 -1.675163083768058e-02  
 1.187525424267582e-01 -1.251251947679634e-01]  
 [1.069896817109715e+00 -3.415185614776689e-13  
 -5.692143405089593e-01 5.272764172438611e-12  
 -1.561208295192408e+00 -3.148587374981679e-12]  
 [7.270527303435753e-01 -1.757729975026406e-13  
 -6.278516618155376e-02 1.661905213936493e-13]



-5.651302536795951e+01 4.629177249859673e-12]  
 [3.198820210487289e-01 7.960341777022914e-13  
 4.011683106895218e-01 -7.270889551785724e-13  
 8.688777340038796e-01 3.187166744173138e-12]  
 [8.387448112864213e-01 5.620028689043277e-01  
 -9.123969777184606e-01 1.675163085017796e-02  
 1.187525423829068e-01 1.251251947713976e-01]  
 [-6.254087204357015e-01 -1.616999448835615e-15  
 2.282818524194373e-01 -9.959131501251217e-14  
 -3.768672392441559e+01 1.639578186760082e-11]  
 [-5.126129685059675e-01 -2.186596579798958e-14  
 6.999395580807085e-01 1.742510487030141e-13  
 1.586644124519027e+01 -3.647423183796017e-11]

13 (conjugate of 10)

[8.513751668930445e-01 -3.887048848155324e-02  
 -7.614121528358986e-01 -2.510696629432730e-02  
 -5.302412002737883e+00 -2.338243159033500e+00]  
 [3.577872337726079e-01 -4.156190715988004e-03  
 3.514127411395447e-01 3.256353440565586e-03  
 1.353433982526609e+00 -2.989672077209169e-02]  
 [-5.187319623376614e-01 7.483489985061595e-04  
 7.169952569709148e-01 5.192950716084680e-04  
 1.110016872117011e+01 -3.229885746120878e-01]  
 [-6.257960072923717e-01 2.238575872891976e-05  
 2.296962485959554e-01 -1.038913191672680e-05  
 -3.752982441660430e+01 2.977171862331144e-03]  
 [-8.921446010559151e-01 -2.315794285686775e-04  
 -3.879777515081767e-01 -1.386521037913054e-06  
 3.788789374189912e+00 -9.467279989432385e-03]  
 [7.144335694864201e-01 3.378160378580521e-04  
 -4.998816961941981e-02 -5.489802761478870e-04  
 -5.439261982637246e+01 -8.198220540473820e-02]  
 [-5.269519643849312e-01 -6.933882091223349e-05  
 -5.560628450599153e-01 -1.401508804779688e-03  
 -1.027656515094413e+01 2.132593095702798e-01]  
 [9.317930943655848e-01 1.472234491577964e-01  
 -8.619742514302801e-01 7.025631110234663e-02  
 -9.898578445501916e-02 1.187108350536902e-01]  
 [7.392493515565261e-01 2.799150198373527e-02  
 -7.773940555783609e-01 -9.409996835984401e-04  
 5.089666486787165e+00 2.751465428200852e+00]  
 [-4.282634374642514e-01 -2.223871485766714e-03  
 -5.040306222168584e-01 -9.651758375418853e-06  
 -8.710731695510239e+00 -2.119998660178265e-01]  
 [9.394960875319655e-01 2.129394010545603e-04  
 -3.043356384839169e-01 3.837627371823798e-04  
 -3.921664398351288e+00 3.495708090546507e-02]  
 [-9.352532350831588e-01 6.157831908363691e-06  
 8.462267205937445e-01 1.501889115596201e-05]

-7.433266615921528e+00 4.353307494558728e-04]  
 [-5.860592499977263e-01 2.210171004137657e-03  
 6.776996385524520e-01 1.233879865051875e-03  
 6.127564458663331e+00 3.187939702202320e-01]  
 [-3.474138835826439e-01 -6.387490855415956e-04  
 -8.813377675335939e-01 7.829948762209116e-04  
 1.422319245769941e+00 1.142150474299108e-02]  
 [8.919571864211296e-01 3.982251035867431e-04  
 -5.068547905984208e-01 -1.975300156681121e-03  
 -4.828796369504440e+01 -4.574428254756299e-01]

14 (conjugate of 7)

[8.278772533392423e-01 -1.232301854883178e-01  
 -7.816330523004066e-01 -2.610950675237492e-02  
 -5.156782959144236e-01 -2.696736260837331e+00]  
 [-9.388894938234230e-01 -9.363491108029137e-04  
 8.479485856457796e-01 8.130430690432488e-05  
 -7.183770940791765e+00 5.232433245351073e-02]  
 [-4.696650194047741e-01 -2.824603317744579e-02  
 -4.822604572529906e-01 7.315078892006781e-02  
 -9.661702837277051e+00 2.140366033386230e+00]  
 [3.354032712715453e-01 3.839074295161987e-03  
 3.797034011321089e-01 -5.043789913949178e-03  
 1.095965811467695e+00 4.855078127998229e-02]  
 [8.925137465232136e-01 -3.853344295395741e-04  
 -5.061567882196544e-01 4.901520505124079e-04  
 -4.841570038935337e+01 1.817311564604051e-01]  
 [-6.742116809265571e-01 1.336807243196173e-02  
 2.754575528981466e-01 -2.939105367589341e-01  
 -6.673025559909174e-01 -3.120559835218356e-01]  
 [-3.442425827707675e-01 3.506713456375922e-02  
 5.613067827438175e-01 4.233475001080364e-02  
 -5.079249888794313e-01 -1.744256126847068e-01]  
 [7.190623422705049e-01 5.209831722317651e-05  
 -5.481170627834693e-02 1.594960169937451e-04  
 -5.533590827504982e+01 -6.497817150198695e-02]  
 [-6.245418856020670e-01 -2.396242989066866e-04  
 2.204039424888478e-01 1.277403194868817e-02  
 -3.613644777426652e+01 8.060940295115036e-01]  
 [-3.647461364609172e-01 -2.475631674669913e-02  
 -8.506455517597330e-01 6.544641081076877e-02  
 1.179807352538258e+00 1.559059183691333e+00]  
 [9.800626946751475e-01 4.730303042902084e-03  
 -3.545152727929674e-01 -1.393915820236987e-02  
 -2.587834666778181e+00 -7.007338479397776e-02]  
 [-9.064590360800469e-01 -3.247602762139072e-03  
 -3.820358825972446e-01 1.927146598281707e-03  
 3.300888201194908e+00 -9.206613577675792e-02]  
 [-4.614020553252697e-01 3.773773537688799e-02  
 -6.278347868166904e-01 -4.251037664696018e-02

-8.544985344387047e+00 -4.238461475673224e+00]  
 [-5.304659519956280e-01 3.312675589842795e-03  
 7.044956246119534e-01 -1.910253193152550e-03  
 1.677227295970988e+01 2.589541409375289e-01]  
 [7.993117848213083e-01 1.337000802750931e-01  
 -7.904881554461144e-01 2.640723811624018e-02  
 1.362304269435987e-01 2.601717367069350e+00]

15 (conjugate of 16)

[-9.365322141444794e-01 1.754750560826120e-02  
 -3.681170222944828e-01 -8.244896339282395e-03  
 2.525384188945623e+00 3.487293935662414e-01]  
 [7.315699475063502e-01 -2.926204949848645e-01  
 -8.262566075321277e-01 -1.433889290352786e-02  
 5.946203896010096e-01 -6.945286759261392e-01]  
 [7.238964388301720e-01 -3.650256343134069e-03  
 -5.954376860835191e-02 3.902436494788862e-03  
 -5.637671804201591e+01 2.848504896424258e-01]  
 [-4.552925910868856e-01 -1.242809885365012e-01  
 -5.596847676618956e-01 6.722314912533892e-02  
 -7.032734537298442e+00 3.147237192566676e+00]  
 [-3.357289432186019e-01 1.986247913557451e-03  
 -9.126002292997374e-01 -4.774779889554407e-03  
 9.815267445879926e-01 -5.638746021267340e-02]  
 [-1.047406736341875e-01 -2.902906852549906e-01  
 4.615298472114333e-01 1.496311102522606e-01  
 -3.233165416948804e-01 -1.127184343778218e-01]  
 [-6.253924390118408e-01 1.824994433547244e-05  
 2.265352354683618e-01 -1.046356973776964e-03  
 -3.745182742293810e+01 6.020095443831597e-02]  
 [9.709912314556743e-01 2.608897068557270e-01  
 -8.190950395355483e-01 8.930849752774592e-02  
 -4.953401084273159e-01 4.049440809009485e-01]  
 [-5.244620941404570e-01 6.041993149309896e-03  
 7.003255012241446e-01 1.097835261012142e-03  
 1.696259611116476e+01 1.152043204541820e-01]  
 [8.934023168127740e-01 -5.063140689181132e-04  
 -5.075419828906479e-01 1.362193000585160e-03  
 -4.884725386419282e+01 1.419190244920295e-01]  
 [3.442597875202250e-01 3.503962770491761e-02  
 3.763460616680533e-01 -3.561163432008856e-02  
 9.829541989843564e-01 1.907040224072171e-01]  
 [-4.950416036585064e-01 1.457220029018768e-01  
 7.416902856783145e-01 8.832425695998647e-02  
 -2.762246872368062e-01 8.051946744250365e-03]  
 [1.053416570830210e+00 -3.595942088023541e-02  
 -4.716199327018319e-01 8.543833788718114e-02  
 -1.620187144550039e+00 -2.883677185829153e-01]  
 [-9.443474823007582e-01 3.899833022422884e-04  
 8.498390519315185e-01 -4.731121016895573e-05]

-6.888554993642763e+00 4.920999617577284e-03]  
 [-4.151554521636688e-01 7.273313113309025e-02  
 -5.540994878171981e-01 -4.903987174196685e-02  
 -9.807015608120887e+00 -3.554760135730313e+00]

16 (conjugate of 15)

[8.934023168126974e-01 5.063140689616066e-04  
 -5.075419828904397e-01 -1.362193000788711e-03  
 -4.884725386416938e+01 -1.419190245001481e-01]  
 [-5.244620941421315e-01 -6.041993149808856e-03  
 7.003255012242520e-01 -1.097835260598537e-03  
 1.696259611111084e+01 -1.152043205647199e-01]  
 -9.443474823003344e-01 -3.899833018899230e-04  
 8.498390519313518e-01 4.731121006627307e-05  
 -6.888554993668300e+00 -4.920999635441795e-03]  
 [7.315699475156253e-01 2.926204949784771e-01  
 -8.262566075304261e-01 1.433889290629690e-02  
 5.946203895733200e-01 6.945286759801543e-01]  
 [3.442597875245219e-01 -3.503962771103571e-02  
 3.763460616638760e-01 3.561163432588742e-02  
 9.829541989993760e-01 -1.907040224369996e-01]  
 [-4.552925910859280e-01 1.242809885300472e-01  
 -5.596847676620120e-01 -6.722314912342686e-02  
 -7.032734537579579e+00 -3.147237192649145e+00]  
 [7.238964388299384e-01 3.650256343268701e-03  
 -5.954376860806512e-02 -3.902436495028595e-03  
 -5.637671804197989e+01 -2.848504896409970e-01]  
 [1.053416570826065e+00 3.595942087937340e-02  
 -4.716199326978093e-01 -8.543833788141445e-02  
 -1.620187144597307e+00 2.883677186195636e-01]  
 [9.709912314458116e-01 -2.608897068552063e-01  
 -8.190950395359942e-01 -8.930849752472346e-02  
 -4.953401084224343e-01 -4.049440809395108e-01]  
 [-4.151554521646167e-01 -7.273313113412476e-02  
 -5.540994878173843e-01 4.903987174364234e-02  
 -9.807015607868868e+00 3.554760135770632e+00]  
 [-1.047406736230291e-01 2.902906852616491e-01  
 4.615298472067544e-01 -1.496311102590321e-01  
 -3.233165416691355e-01 1.127184343700080e-01]  
 [-6.253924390118348e-01 -1.824994434412787e-05  
 2.265352354682418e-01 1.046356973713953e-03  
 -3.745182742293368e+01 -6.020095442750040e-02]  
 [-9.365322141431210e-01 -1.754750560664212e-02  
 -3.681170222950526e-01 8.244896338463488e-03  
 2.525384188980222e+00 -3.487293935421025e-01]  
 [-4.950416036394085e-01 -1.457220029166762e-01  
 7.416902856974044e-01 -8.832425694799610e-02  
 -2.762246871915444e-01 -8.051946619675303e-03]  
 [-3.357289432184485e-01 -1.986247913551390e-03  
 -9.126002293001843e-01 4.774779889841355e-03]

9.815267445821356e-01 5.638746021587525e-02]

An example of real identifiable tensor of type  $\mathbb{P}^2 \times \mathbb{P}^4 \times \mathbb{P}^9$ :  
with the notation of the paper, assuming that  $L$  is the real linear space of dimension 8 spanned by the real rank-1 tensors of  $\mathbb{P}^2 \times \mathbb{P}^4$  given by

$$M_1 = (1, 547, 26, 218, 235) \otimes (1, -179, 513)$$

$$M_2 = (1, -525, 314, 543, 496) \otimes (1, 291, 523)$$

$$M_3 = (1, 382, 202, 475, -431) \otimes (1, 267, 410)$$

$$M_4 = (1, 254, 315, -137, 378) \otimes (1, 243, 498)$$

$$M_5 = (1, -365, 473, 298, 437) \otimes (1, 4, 234)$$

$$M_6 = (1, 144, 190, 280, 150) \otimes (1, 17, 81)$$

$$M_7 = (1, 288, 545, 450, -17) \otimes (1, 485, -69)$$

$$M_8 = (1, 385, 235, -514, 13) \otimes (1, 52, 526)$$

$$M_9 = (1, 187, -113, 437, 15) \otimes (1, 506, 504)$$

by computing, with the aid of the software system Macaulay2 (see the script at the end), the eigenvalues and the eigenvectors of certain *companion* matrices, we get that

$$X \cap L = \{M_1, M_2, M_3, M_4, M_5, M_6, M_7, M_8, M_9, M_{10}, M_{11}, M_{12}, M_{13}, M_{14}, M_{15}\}$$

where

$$M_{10} = \begin{pmatrix} 1 & \star & \star \\ \star & \star & \star \\ \star & 16202.1 + 70354.9i & 77275 + 45608.2i \\ 286.582 - 12.4463i & -6076.83 + 59269.2i & 48217.2 + 56200.3i \\ 303.855 - 133.903i & 18362.7 + 66478.4i & 75630.4 + 40343.3i \end{pmatrix}, M_{11} = \overline{M_{10}}$$

$$M_{12} = \begin{pmatrix} 1 & \star & \star \\ \star & \star & \star \\ \star & 52613 + 39556.3i & 124001 + 48847.5i \\ -309.435 - 74.0458i & -69868 - 37138.2i & -156374 - 34829.3i \\ 229.189 + 153.645i & 45582.3 - 51291.5i & 116604 + 75539.8i \end{pmatrix}, M_{13} = \overline{M_{12}}$$

$$M_{14} = \begin{pmatrix} 1 & \star & \star \\ \star & \star & \star \\ \star & 2938.16 + 10097.7i & 2554.88 + 6586.39i \\ 237.235 + 1.3350i & 122538 + 76331.2i & 86454.6 + 43940.2i \\ 71.3692 - 57.1638i & 55291.8 - 6252.04i & 36638.3 - 7406.94i \end{pmatrix}, M_{15} = \overline{M_{14}}$$

are non-real rank-1 tensors of  $\mathbb{P}^2 \times \mathbb{P}^4$  (in the above matrices, the symbol  $\star$  denotes entries that can be easily computed from the other ones using the rank-1 property).

The script of our algorithm is the following:

```

k=QQ;
R=k[x_0..x_14];
n = 560;
l1 = for i from 0 to 5 list random(n);
l2 = for i from 0 to 5 list random(n);
l3 = for i from 0 to 5 list random(n);
l4 = for i from 0 to 5 list random(n);
l5 = for i from 0 to 5 list random(n);
l6 = for i from 0 to 5 list random(n);
l7 = for i from 0 to 5 list random(n);
l8 = for i from 0 to 5 list random(n);
l9 = for i from 0 to 5 list random(n);
M1 = (transpose(matrix(R,{{1,l1_2,l1_3,l1_4,l1_5}})))*(matrix(R,{{1,l1_0,l1_1}}));
M2 = (transpose(matrix(R,{{1,l2_2,l2_3,l2_4,l2_5}})))*(matrix(R,{{1,l2_0,l2_1}}));
M3 = (transpose(matrix(R,{{1,l3_2,l3_3,l3_4,l3_5}})))*(matrix(R,{{1,l3_0,l3_1}}));
M4 = (transpose(matrix(R,{{1,l4_2,l4_3,l4_4,l4_5}})))*(matrix(R,{{1,l4_0,l4_1}}));
M5 = (transpose(matrix(R,{{1,l5_2,l5_3,l5_4,l5_5}})))*(matrix(R,{{1,l5_0,l5_1}}));
M6 = (transpose(matrix(R,{{1,l6_2,l6_3,l6_4,l6_5}})))*(matrix(R,{{1,l6_0,l6_1}}));
M7 = (transpose(matrix(R,{{1,l7_2,l7_3,l7_4,l7_5}})))*(matrix(R,{{1,l7_0,l7_1}}));
M8 = (transpose(matrix(R,{{1,l8_2,l8_3,l8_4,l8_5}})))*(matrix(R,{{1,l8_0,l8_1}}));
M9 = (transpose(matrix(R,{{1,l9_2,l9_3,l9_4,l9_5}})))*(matrix(R,{{1,l9_0,l9_1}}));
M = ((M1^{0}|M1^{1}|M1^{2}|M1^{3}|M1^{4}) || (M2^{0}|M2^{1}|M2^{2}|M2^{3}|M2^{4}) ||
      (M3^{0}|M3^{1}|M3^{2}|M3^{3}|M3^{4}) || (M4^{0}|M4^{1}|M4^{2}|M4^{3}|M4^{4}) ||
      (M5^{0}|M5^{1}|M5^{2}|M5^{3}|M5^{4}) || (M6^{0}|M6^{1}|M6^{2}|M6^{3}|M6^{4}) ||
      (M7^{0}|M7^{1}|M7^{2}|M7^{3}|M7^{4}) || (M8^{0}|M8^{1}|M8^{2}|M8^{3}|M8^{4}) ||
      (M9^{0}|M9^{1}|M9^{2}|M9^{3}|M9^{4}));
P5 = gens(ker M);
P8 = ideal((vars R)*P5_{0},(vars R)*P5_{1},(vars R)*P5_{2},(vars R)*P5_{3},
           (vars R)*P5_{4},(vars R)*P5_{5});
N = genericMatrix(R,x_0,3,5);
J = ideal(gens P8,gens minors(2,N),matrix{{x_0-1}});
dim J
degree J
S = R/J;
B = basis S;
BB = sub(B,R);
comp7 = sub(contract(transpose BB,(BB_(0,0))*sub(x_7,R)%J),{sub(x_7,R)=>0_k,
sub(x_8,R)=>0_k,sub(x_9,R)=>0_k,sub(x_10,R)=>0_k,sub(x_11,R)=>0_k,
sub(x_12,R)=>0_k,sub(x_13,R)=>0_k,sub(x_14,R)=>0_k});
for i from 1 to 14 do
comp7 = comp7|sub(contract(transpose BB,(BB_(0,i))*sub(x_7,R)%J),{sub(x_7,R)=>0_k,
sub(x_8,R)=>0_k,sub(x_9,R)=>0_k,sub(x_10,R)=>0_k,sub(x_11,R)=>0_k,
sub(x_12,R)=>0_k,sub(x_13,R)=>0_k,sub(x_14,R)=>0_k});
comp7 = sub(comp7,RR);
comp7t = transpose(comp7);
comp8 = sub(contract(transpose BB,(BB_(0,0))*sub(x_8,R)%J),{sub(x_7,R)=>0_k,
sub(x_8,R)=>0_k,sub(x_9,R)=>0_k,sub(x_10,R)=>0_k,sub(x_11,R)=>0_k,
sub(x_12,R)=>0_k,sub(x_13,R)=>0_k,sub(x_14,R)=>0_k});
for i from 1 to 14 do
comp8 = comp8|sub(contract(transpose BB,(BB_(0,i))*sub(x_8,R)%J),{sub(x_7,R)=>0_k,

```

```

sub(x_8,R)=>0_k,sub(x_9,R)=>0_k,sub(x_10,R)=>0_k,sub(x_11,R)=>0_k,
sub(x_12,R)=>0_k,sub(x_13,R)=>0_k,sub(x_14,R)=>0_k});
comp8 = sub(comp8,RR);
comp8t = transpose(comp8);
comp9 = sub(contract(transpose BB, (BB_(0,0))*sub(x_9,R)%J), {sub(x_7,R)=>0_k,
sub(x_8,R)=>0_k,sub(x_9,R)=>0_k,sub(x_10,R)=>0_k,sub(x_11,R)=>0_k,
sub(x_12,R)=>0_k,sub(x_13,R)=>0_k,sub(x_14,R)=>0_k});
for i from 1 to 14 do
comp9 = comp9|sub(contract(transpose BB, (BB_(0,i))*sub(x_9,R)%J), {sub(x_7,R)=>0_k,
sub(x_8,R)=>0_k,sub(x_9,R)=>0_k,sub(x_10,R)=>0_k,sub(x_11,R)=>0_k,
sub(x_12,R)=>0_k,sub(x_13,R)=>0_k,sub(x_14,R)=>0_k});
comp9 = sub(comp9,RR);
comp9t = transpose(comp9);
comp10 = sub(contract(transpose BB, (BB_(0,0))*sub(x_10,R)%J), {sub(x_7,R)=>0_k,
sub(x_8,R)=>0_k,sub(x_9,R)=>0_k,sub(x_10,R)=>0_k,sub(x_11,R)=>0_k,
sub(x_12,R)=>0_k,sub(x_13,R)=>0_k,sub(x_14,R)=>0_k});
for i from 1 to 14 do
comp10 = comp10|sub(contract(transpose BB, (BB_(0,i))*sub(x_10,R)%J), {sub(x_7,R)=>0_k,
sub(x_8,R)=>0_k,sub(x_9,R)=>0_k,sub(x_10,R)=>0_k,sub(x_11,R)=>0_k,
sub(x_12,R)=>0_k,sub(x_13,R)=>0_k,sub(x_14,R)=>0_k});
comp10 = sub(comp10,RR);
comp10t = transpose(comp10);
comp11 = sub(contract(transpose BB, (BB_(0,0))*sub(x_11,R)%J), {sub(x_7,R)=>0_k,
sub(x_8,R)=>0_k,sub(x_9,R)=>0_k,sub(x_10,R)=>0_k,sub(x_11,R)=>0_k,
sub(x_12,R)=>0_k,sub(x_13,R)=>0_k,sub(x_14,R)=>0_k});
for i from 1 to 14 do
comp11 = comp11|sub(contract(transpose BB, (BB_(0,i))*sub(x_11,R)%J), {sub(x_7,R)=>0_k,
sub(x_8,R)=>0_k,sub(x_9,R)=>0_k,sub(x_10,R)=>0_k,sub(x_11,R)=>0_k,
sub(x_12,R)=>0_k,sub(x_13,R)=>0_k,sub(x_14,R)=>0_k});
comp11 = sub(comp11,RR);
comp11t = transpose(comp11);
comp12 = sub(contract(transpose BB, (BB_(0,0))*sub(x_12,R)%J), {sub(x_7,R)=>0_k,
sub(x_8,R)=>0_k,sub(x_9,R)=>0_k,sub(x_10,R)=>0_k,sub(x_11,R)=>0_k,
sub(x_12,R)=>0_k,sub(x_13,R)=>0_k,sub(x_14,R)=>0_k});
for i from 1 to 14 do
comp12 = comp12|sub(contract(transpose BB, (BB_(0,i))*sub(x_12,R)%J), {sub(x_7,R)=>0_k,
sub(x_8,R)=>0_k,sub(x_9,R)=>0_k,sub(x_10,R)=>0_k,sub(x_11,R)=>0_k,
sub(x_12,R)=>0_k,sub(x_13,R)=>0_k,sub(x_14,R)=>0_k});
comp12 = sub(comp12,RR);
comp12t = transpose(comp12);
comp13 = sub(contract(transpose BB, (BB_(0,0))*sub(x_13,R)%J), {sub(x_7,R)=>0_k,
sub(x_8,R)=>0_k,sub(x_9,R)=>0_k,sub(x_10,R)=>0_k,sub(x_11,R)=>0_k,
sub(x_12,R)=>0_k,sub(x_13,R)=>0_k,sub(x_14,R)=>0_k});
for i from 1 to 14 do
comp13 = comp13|sub(contract(transpose BB, (BB_(0,i))*sub(x_13,R)%J), {sub(x_7,R)=>0_k,
sub(x_8,R)=>0_k,sub(x_9,R)=>0_k,sub(x_10,R)=>0_k,sub(x_11,R)=>0_k,
sub(x_12,R)=>0_k,sub(x_13,R)=>0_k,sub(x_14,R)=>0_k});
comp13 = sub(comp13,RR);
comp13t = transpose(comp13);
comp14 = sub(contract(transpose BB, (BB_(0,0))*sub(x_14,R)%J), {sub(x_7,R)=>0_k,

```

```

        sub(x_8,R)=>0_k,sub(x_9,R)=>0_k,sub(x_10,R)=>0_k,sub(x_11,R)=>0_k,
        sub(x_12,R)=>0_k,sub(x_13,R)=>0_k,sub(x_14,R)=>0_k});
for i from 1 to 14 do
comp14 = comp14|sub(contract(transpose BB,(BB_(0,i))*sub(x_14,R)%J),{sub(x_7,R)=>0_k,
        sub(x_8,R)=>0_k,sub(x_9,R)=>0_k,sub(x_10,R)=>0_k,sub(x_11,R)=>0_k,
        sub(x_12,R)=>0_k,sub(x_13,R)=>0_k,sub(x_14,R)=>0_k});
comp14 = sub(comp14,RR);
comp14t = transpose(comp14);
eigenvectors comp14t
eigenvectors comp14t
eigenvectors comp14t
eigenvectors comp14t
eigenvectors comp14t
eigenvectors comp14t
eigenvectors comp14t
eigenvectors comp14t
eigenvectors comp14t

```

(E. Angelini, C. Bocci, L. Chiantini) DIPARTIMENTO DI INGEGNERIA DELL'INFORMAZIONE E SCIENZE MATEMATICHE,  
 UNIVERSITÀ DI SIENA, VIA ROMA 56, 53100 SIENA, ITALIA  
*E-mail address:* elena.angelini@unisi.it, cristiano.bocci@unisi.it, luca.chiantini@unisi.it
